# Supplementary material for: MeshMimic: Geometry-Aware Humanoid Motion Learning through 3D Scene Reconstruction
Source: arXiv:2602.15733 source file (2026-02-17)
Supplement: Supplementary file 1 [file supplementary.tex]

\section{Evaluation Details}
\label{app:eval_details}

For quantitative evaluation of our real-to-sim pipeline, we conduct experiments on the SLOPER4D dataset~\cite{sloper4d}.
Following established protocols~\cite{videomimic,wham,tram}, we assess human trajectory reconstruction using
World-frame Mean Per Joint Position Error (W-MPJPE) and World-frame Aligned MPJPE (WA-MPJPE),
and evaluate scene geometry reconstruction using the Chamfer Distance.

\paragraph{Human trajectory metrics.}
For each sequence, we partition the motion into 100-frame segments.
To emphasize global consistency, W-MPJPE is computed after aligning only the first two frames of each segment to the ground truth.
In contrast, WA-MPJPE aligns the entire segment, thereby measuring local trajectory accuracy over time.

\paragraph{Scene geometry metric.}
For geometry evaluation, we compute the Chamfer Distance (in meters) between the aligned predicted point cloud and the LiDAR point cloud,
restricted to the RGB camera's field of view.

\paragraph{Benchmark subset and baselines.}
For benchmarking, we use a subset of SLOPER4D that includes only sequences where SAM2 tracking---comprising human detection and
cross-frame association---is successful. This subset contains two sequences for each activity category: running, walking, and stair
ascent/descent. Results for VideoMimic, WHAM and TRAM are reproduced using their official implementations.
